# Supplementary material for: Consistent Approximations for the Optimal Control of Constrained Switched Systems
Source: arXiv:1208.0062 source file (2012-08-19)
Supplement: Supplementary file 1 [file appendix.tex]

\section{Set-Valued Function Properties}

	\begin{definition}
		Let ${\cal X}$ be a metric space. A function $f: {\cal X} \to \R$ is \emph{upper semi-continuous at $\hat{x}$} if for any sequence $\{x_i\}_{i=0}^{\infty} \subset {\cal X}$ such that $x_i \to \hat{x}$ as $i \to \infty$, $\limsup f(x_i) \leq f(\hat{x})$. A function is called \emph{upper semi-continuous} if is upper semi-continuous for all $x \in {\cal X}$. A function $f: {\cal X} \to \R$ is \emph{lower semi-continuous at $\hat{x}$} if for any sequence $\{x_i\}_{i=0}^{\infty} \subset {\cal X}$ such that $x_i \to \hat{x}$ as $i \to \infty$, $\liminf f(x_i) \geq f(\hat{x})$. A function is called \emph{lower semi-continuous} if is lower semi-continuous for all $x \in {\cal X}$. A function is \emph{continuous} if it is both upper and lower semi-continuous.
	\end{definition}
	
\begin{lemma}
	\label{lemma:max_usc}
	 Let ${\cal X}$ be a metric space. Let $f,g: {\cal X} \to \R$ be upper semi-continuous, then the point-wise maximum of $f$ and $g$ is upper semi-continuous. 
\end{lemma}
\begin{proof}
	Since $f$ and $g$ are upper semi-continuous, we know for each $x_0 \in {\cal X}$ and for every $\epsilon > 0$ there exists neighborhoods $U_f$ and $U_g$ of $x$ such that $f(x) \leq f(x_0) + \epsilon$ for all $x \in U_f$ and $g(x) \leq g(x_0) + \epsilon$ for all $x \in U_g$. To show that $\max\{f,g\}$ is upper semi-continuous, for each $x_0 \in {\cal X}$ and for every $\epsilon > 0$, we choose a neighborhood $U_{fg} = U_f \cap U_g$ and show that $\max\{f(x),g(x)\} \leq \max\{f(x_0),g(x_0)\} + \epsilon$ for all $x \in U_{f,g}$. 
	
	We need only consider two cases: $\max\{f(x),g(x)\} = f(x)$ for all $x \in U_{fg}$ or $\max\{f(x_0),g(x_0)\} = f(x_0)$ but $\max\{f(x),g(x)\} = g(x)$ for some $x \in U_{fg}$. The result in the first case is obvious. In the second case, notice $g(x) - f(x_0) \geq f(x) - f(x_0)$ since $g(x) \geq f(x)$ and $g(x) - f(x_0) \leq g(x) - g(x_0)$ since $f(x_0) \geq g(x_0)$. So $g(x) - f(x_0) \leq \max\{f(x)- f(x_0),g(x) - g(x_0)\} \leq \epsilon$ for all $x \in U_{fg}$ which proves our result. 
\end{proof}
	
	\begin{definition}
		Let ${\cal X}$ be a metric space. Consider a sequence of sets $\{X_i\}_{i=0}^{\infty}$ in ${\cal X}$. Denote the set of limit points of $\{X_i\}_{i=0}^{\infty}$ by $\uline{\lim}\, X_i$ and call it the \emph{inner limit}. Denote the set of cluster points of $\{X_i\}_{i=0}^{\infty}$ by $\overline{\lim}\, X_i$ and call it the \emph{outer limit}.
	\end{definition}
	
	\begin{definition}
	Let ${\cal X}$ and ${\cal Y}$ be metric spaces. A function $f: {\cal X} \to 2^{\cal Y}$ is \emph{outer semi-continuous at $\hat{x}$} if for any sequence $\{x_i\}_{i=0}^{\infty}$ such that $x_i \to \hat{x}$ as $i \to \infty$, $\overline{\lim} f(x_i) \subset f(\hat{x})$. A function is \emph{outer semi-continuous} if it is upper semi-continuous for all $x \in {\cal X}$. A function $f: {\cal X} \to 2^{\cal Y}$ is \emph{inner semi-continuous at $\hat{x}$} if for any sequence $\{x_i\}_{i=0}^{\infty}$ such that $x_i \to \hat{x}$ as $i \to \infty$, $\uline{\lim} f(x_i) \supset f(\hat{x})$. A function is \emph{inner semi-continuous} if it is inner semi-continuous for all $x \in {\cal X}$. A function is \emph{continuous} if it is both inner and outer semi-continuous.
	\end{definition}
	
	Note that, when $f: {\cal X} \to {\cal Y}$ is either outer semi-continuous and locally bounded, then it is continuous in the ordinary (as opposed to set-valued) sense.
	
	\begin{lemma}
		\label{lemma:psi_upper_semi_continuous}
		Let ${\cal X}$ and ${\cal Y}$ be metric spaces. Suppose that $\phi:{\cal X} \times {\cal Y} \to \R$ is continuous, that $Y:{\cal X} \to 2^{\cal Y}$ is outer semi-continuous, and that the function $\psi:{\cal X} \to \R$ defined by
		\begin{equation}
			\label{eq:psi}
			\psi(x) = \max_{y \in Y(x)} \phi(x,y)
		\end{equation}
		is well defined for all $x \in {\cal X}$. If, for every bounded set $X \subset {\cal X}$, there exists an $\alpha < \infty$ such that for all $x \in X$, 
		\begin{equation}
			\label{eq:bound}
			\left\| \arg \max_{y \in Y(x)} \phi(x,y) \right\| \leq \alpha,
		\end{equation}
		then $\psi(\cdot)$ is upper semi-continuous.
	\end{lemma}
\begin{proof}
	Let $\hat{x} \in {\cal X}$ be given. Let $\{x_i\}_{i=0}^{\infty}$ be an arbitrary sequence converging to $\hat{x}$, and let $y_i \in Y(x_i)$ be such that $\psi(x_i) = \phi(x_i,y_i)$. Since the sequence $\{x_i\}_{i=0}^{\infty}$ is bounded, it follows that there exists an $\alpha < \infty$ such that $\|y_i\| \leq \alpha$ for all $i \in \N$ and hence because $\phi(\cdot,\cdot)$ is continuous, $\overline{\lim}_{i\to\infty} \phi(x_i,y_i)$ exists. We can take a subsequence of $\{y_i\}_{i=0}^{\infty}$ such that $\overline{\lim}\,\phi(x_i,y_i) = \lim_{j\to\infty}\phi(x_{i_j},y_{i_j})$ and $y_{i_j} \to y^*$ as $j \to \infty$. Then $y^* \in Y(\hat{x})$ because $Y(\cdot)$ is outer semi-continuous and hence:
	\begin{equation}
		\psi(\hat{x}) \geq \phi(\hat{x},y^*) = \overline{\lim}_{i\to\infty} \psi(x_i),
	\end{equation}
	which completes our proof.
\end{proof}

	\begin{lemma}
		\label{lemma:max_continuous}
		Suppose that $\phi: {\cal X} \times {\cal Y} \to \R$ is continuous, that $Y: {\cal X} \to 2^{\cal Y}$ is continuous and that the function $\psi: {\cal X} \to \R$, defined by Equation \eqref{eq:psi}, is well defined for all $x \in {\cal X}$. If for every bounded set $X \subset {\cal X}$, there exists and $\alpha < \infty$ such that Equation \eqref{eq:bound} holds for all $x \in X$, then $\psi(\cdot)$ defined by Equation \eqref{eq:psi} is continuous. 
		
		Furthermore, if in addition $Y(x) = Y$, where $Y \subset {\cal Y}$ is a compact set and $\phi(\cdot,y)$ is Lipschitz continuous on bounded sets, then $\psi(\cdot)$, defined by Equation \eqref{eq:psi} is Lipschitz continuous on bounded sets.
		
	\end{lemma}
	\begin{proof}
		Given the previous result, we need only show that $\psi(\cdot)$ is lower semi-continuous. For the sake of contradiction, suppose that there is a point $\hat{x} \in {\cal X}$ and a sequence $\{x_i\}_{i=0}^{\infty}$ converging to $\hat{x}$ such that $\lim\,\psi(x_i)$ exists and $\lim \, \psi(x_i) < \psi (\hat{x})$. Suppose that $\psi(\hat{x}) = \phi(\hat{x},\hat{y})$ with $\hat{y} \in Y(\hat{x})$. Since $Y(\cdot)$ is continuous, there exists $y_i \in Y(x_i)$ such that $y_i \to \hat{y}$ as $i \to \infty$. Since $\phi(\cdot,\cdot)$ is continuous, $\lim_{i\to\infty}\phi(x_i,y_i) = \phi(\hat{x},\hat{y})$. Hence there exists an $i_0$ such that $\phi(x_i,y_i) \geq \psi(x_i)$ for all $i \geq i_0$ which contradicts the definition of $\psi(x_i)$.
		
		Now suppose that $Y(x) = Y$, a compact set, and that $\phi(\cdot,y)$ is Lipschitz continuous on bounded sets. Let $S \subset {\cal X}$ be a bounded set. Since $Y$ is compact, there exists a Lipschitz constant $L < \infty$ such that:
		\begin{equation}
			\left|\phi(x',y) - \phi(x'',y) \right| \leq L \left\|x' - x'' \right\|_{\cal X},
		\end{equation}
		for any $x',x'' \in S$ and all $y\in Y$. Hence:
		\begin{equation}
			\psi(x') - \psi(x'') \leq \max_{y \in Y}\{\phi(x',y) -\phi(x'',y) \} \leq L\left\| x' - x'' \right\|_{\cal X}.
		\end{equation}
		Reversing the roles of $x'$ and $x''$ in the above equation, we obtain the desired result.
	\end{proof}
	
	\begin{lemma}
		\label{lemma:minimizer_continuous}
		Consider the function
		\begin{equation}
			\psi(x) = \max_{y \in Y(x)} \phi(x,y)
		\end{equation}
		with $\phi:{\cal X} \times {\cal Y} \to \R$ continuous and $Y:{\cal X} \to 2^{\cal Y}$ continuous and compact-valued. Let 
		\begin{equation}
			\hat{Y}(x) = \{y \in Y(x) \mid \psi(x) = \phi(x,y) \}.
		\end{equation}
		Then $\hat{Y}(\cdot)$ is outer semi-continuous and compact-valued. Furthermore, if $\hat{Y}(x) = \{\hat{y}(x)\}$, a singleton then $\hat{y}(\cdot)$ is continuous at $x$.
	\end{lemma}
	\begin{proof}
		Clearly, $\hat{Y}(\cdot)$ is compact-valued because $\phi(\cdot,\cdot)$ is continuous and $Y(\cdot)$ is compact-valued. Suppose that $\hat{Y}(\cdot)$ is not outer semi-continuous, then there exists a point $\hat{x}$ and a sequence $x_i \to \hat{x}$ as $i \to \infty$ such that for some $y_i \in \hat{Y}(x_i)$, $y_i \to \hat{y} \notin \hat{Y}(\hat{x})$ as $i \to \infty$. But this means that $\psi(x_i) = \phi(x_i,y_i) \to \phi(\hat{x},\hat{y}) < \psi(\hat{x})$, as $i \to \infty$ which contradicts the continuity of $\psi(\cdot)$. When $\hat{Y}(x)$ is a singleton, its continuity follows directly from the definition of outer semi-continuity and the fact that it is bounded. 
	\end{proof}
